# Supplementary material for: A Label is Worth a Thousand Images in Dataset Distillation
Source: arXiv:2406.10485 source file (2025-01-19)
Supplement: Supplementary file 1 [file waste_bin.tex]

\section{No longer needed, waste bin}
Take aways from this section:
\begin{itemize}
    \item We can perform the same post-hoc label tagging strategy on synthetic images generated by distillation algorithm and still observe a performance boost (Table \ref{tab:softlabel_synthetic}).
    \item Compared to randomly sampled training data, softlabels on those synthetic images have much lower entropy, and hence the performance boost is weaker. (For example, Figure \ref{fig:softmax_density_mtt})
\end{itemize}

\begin{figure}[h]
    \centering
    \includegraphics[width=.5\textwidth]{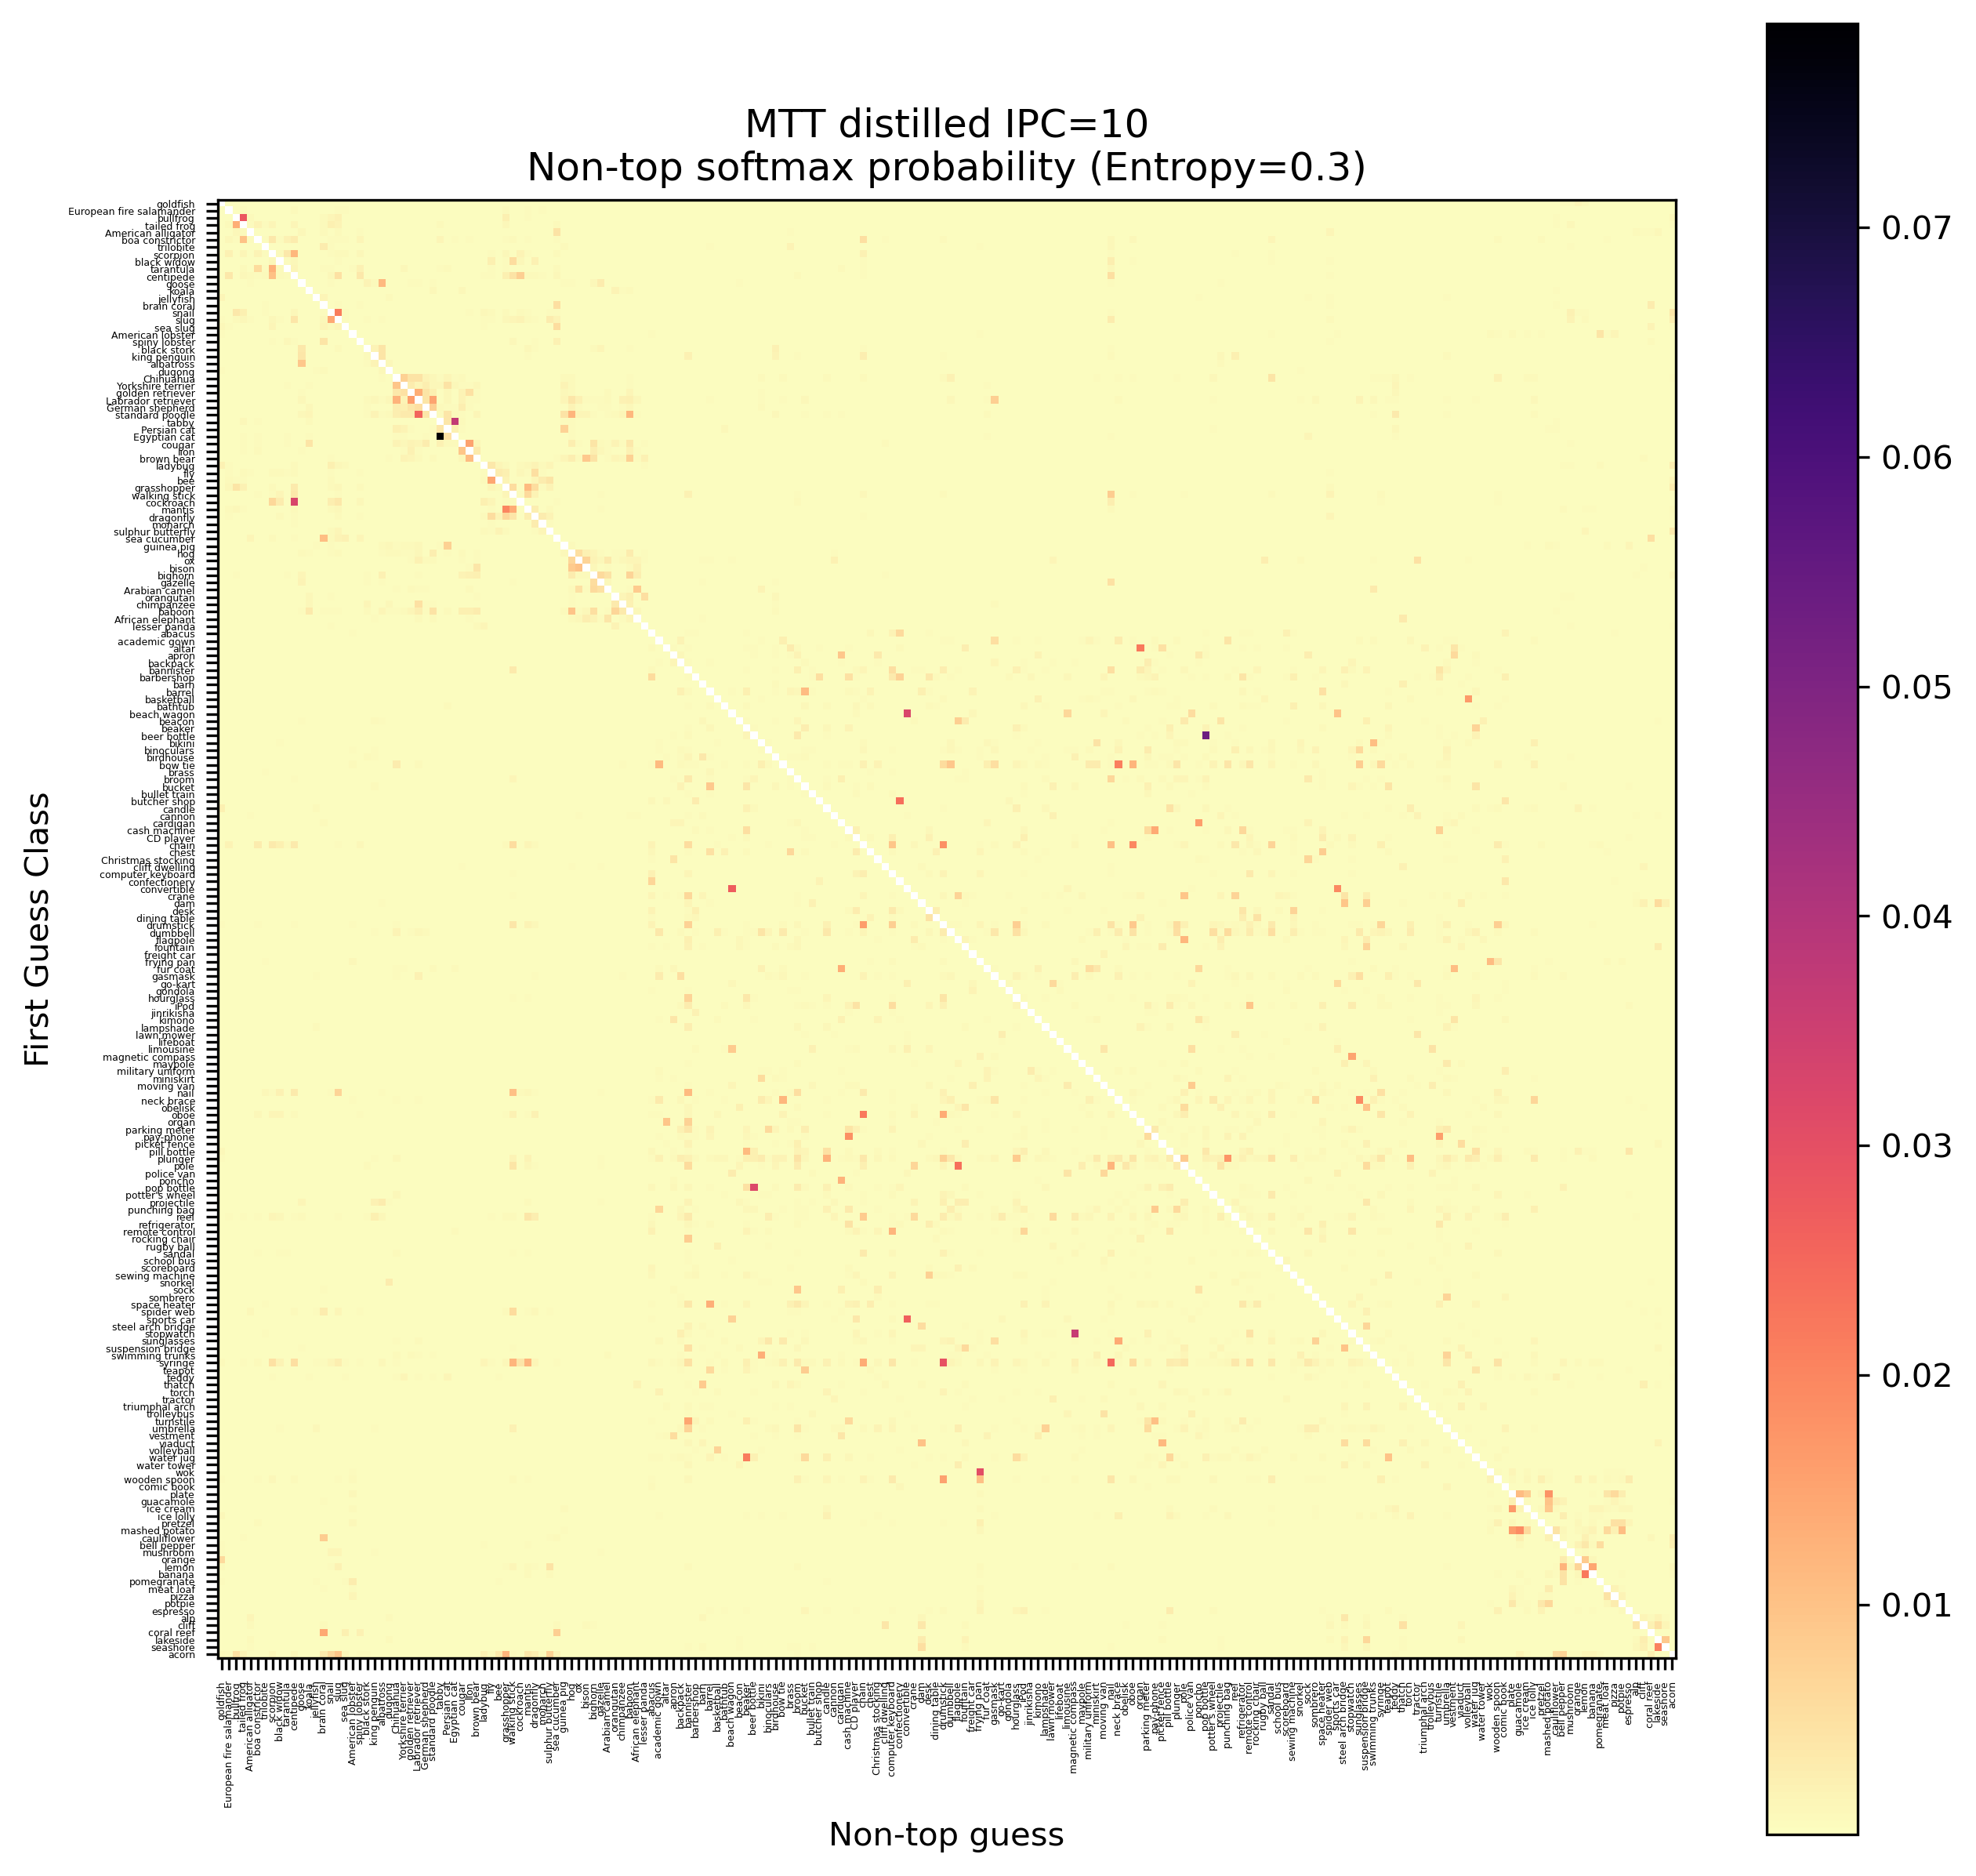}
    \caption{\textbf{Visualizing softmax probabilities for each class in Tiny ImageNet} Softlabels are generated by experts on images generarted by MTT. The class similarity is lost in MTT generated images}
    \label{fig:softmax_density_mtt}
\end{figure}

\begin{table*}[h]
% \parbox{.7\linewidth}{
\centering
\caption{\textbf{Data distillation methods benefit from direct softlabel tagging}}
\label{tab:softlabel_synthetic}
\resizebox{.6\columnwidth}{!}{

\begin{tabular}{@{\extracolsep{0pt}}c cccc cccc}
\toprule    
     Image  & \multicolumn{2}{c}{\textbf{Ra-BPTT}}  & \multicolumn{2}{c}{\textbf{MTT}} & \multicolumn{2}{c}{\textbf{Train}}   \\
     \cmidrule(lr){2-3}  \cmidrule(lr){4-5}    \cmidrule(lr){6-7}  
     Label  &  Hard label & Softlabel & Hard label & Softlabel  & Hard label & Softlabel \\
    \midrule
    IPC=1 & \errbar{8.6}{}& \errbar{}{}& \errbar{8.4}{} & \errbar{11.3}{} & \errbar{1.6}{0.1}& \errbar{7.6}{} \\
    10 & \errbar{15.4}{}& \errbar{}{}& \errbar{23.2}{}& \errbar{27.6}{} & \errbar{6.2}{0.2}& \errbar{27.2}{} \\
    50 & \errbar{}{}& \errbar{}{}& \errbar{28.1}{}& \errbar{33.8}{} & \errbar{21.7}{}& \errbar{35.6}{}\\
\bottomrule
\end{tabular}}
\end{table*}
